# Supplementary material for: OpenBA: An Open-sourced 15B Bilingual Asymmetric seq2seq Model Pre-trained from Scratch
Source: arXiv:2309.10706 source file (2023-10-01)
Supplement: Supplementary file 1 [file Contribution.tex]

\section{Contributions}
\label{sec:contributions}
In this section, we list the contributions of all the participants.

% \textbf{Algorithm:} 

% \textbf{Data:}

% \textbf{Technique Advice:} Wenliang Chen, Guohong Fu, Qiaoming Zhu, Guodong Zhou, Min Zhang

\paragraph{ Project Leader:} Juntao Li
\paragraph{Model Training and Implementation}
\begin{itemize}
    \item \textbf{Model Implementation:} Yuyang Ding, Zecheng Tang, Pinzheng Wang
    \item \textbf{Large-Scale Training \& Monitoring:} Zecheng Tang, Pinzheng Wang, Yuyang Ding
    \item \textbf{Model Architecture:} Zecheng Tang, Yuyang Ding, Pinzheng Wang
    \item \textbf{Training Stability:} Yuyang Ding, Zecheng Tang, Pinzheng Wang
    \item \textbf{Training \& Inference Efficiency:} Yuyang Ding, Pinzheng Wang, Zecheng Tang
    \item \textbf{Model Performance Validation:} Pinzheng Wang, Zecheng Tang, Yuyang Ding
    
\end{itemize}

\paragraph{Data Collection and Processing}
\begin{itemize}
    \item \textbf{Pre-training Data Processing \& Filtering:} Pinzheng Wang, Zecheng Tang, Yuyang Ding 
    \item \textbf{Chinese Flan Dataset Collection \& Filtering:} Pei Guo, Zecheng Tang, Wangjie You 
    \item \textbf{BiFlan Dataset Combination \& Filtering:} Pingzheng Wang, Zecheng Tang, Pei Guo
\end{itemize}

\paragraph{Evaluation and Demo}
\begin{itemize}
    \item \textbf{Evaluation Framework \& Experiments:} Pinzheng Wang, Yuyang Ding, Zecheng Tang
    \item \textbf{Github \& API:} Zecheng Tang, Yuyang Ding, Dan Qiao, Pinzheng Wang 
\end{itemize}

\paragraph{Manuscript Writing and Others:}
\begin{itemize}
    \item \textbf{Manuscript Writing:} Zecheng Tang, Juntao Li, Yuyang Ding, Pei Guo, Pinzheng Wang
    \item \textbf{Figure Design:} Zecheng Tang, Wangjie You, Pingzheng Wang
\end{itemize}

\paragraph{Computation Sponsor}
\begin{itemize}
    \item \textbf{GPU Sponsor:} Min Zhang, Guodong Zhou, Qiaoming Zhu, Wenliang Chen, Guohong Fu
    % \item \textbf{Datasets Provider:} ChaoLang, Yu Hong
\end{itemize}
